# Supplementary material for: Geometric effects induce anomalous size-dependent active transport in structured environments
Source: arXiv:2010.12115 ancillary file (2022-06-17)
Supplement: Supplementary file 1 [file SI_CQGL2022.pdf]

# Supplementary Material: Geometric effects induce anomalous size-dependent active transport in structured environments

Pooja Chopra, David Quint, Ajay Gopinathan, and Bin Liu
*Department of Physics, University of California, 5200 North Lake Road, Merced, CA 95343*

## Geometric constraints

The effective attraction and repulsion of a circular pillar on a circulating bacterium are determined by the orientation of the cell relative to the nearest-neighbor pillar $\theta_p$ (Fig. 3). Given the lattice geometry, such an orientation can be shown as a function of the cell's position, here the angular position $\gamma$ with respect to the center of the orbited pillar. We show in the following that such a function can be solved analytically.

In this analytical model, we consider the whole body of the bacterium (including the flagellar bundle) an infinitely thin rod (thick line) that is only allowed to move in the $x$-$y$ plane (Fig. S1). For a cell that orbits a pillar (centered at $O$ and sitting on a square lattice with lateral size $a = |\overrightarrow{OO'}|$), the leading edge of the rod contacts the pillar's circumference at the point $A$ with an angle $\gamma$, i.e., $\overrightarrow{OA} = (R\cos\gamma, R\sin\gamma)$. Here, we allow the cell orientation to deviate from the surface tangent by an incident angle $\theta_i$ [1, 2]. An elongation of the rod along the trailing edge intersects the nearest-neighbor pillar (centered at $O'$) at the point $A'$ with an angle $\gamma'$ with respect to that pillar, i.e., $\overrightarrow{OA'} = \big(a + R\cos\gamma', R\sin\gamma'\big)$, subject to its geometric constraints. The rotation of the vector $\overrightarrow{AA'}$ from the surface normal of the pillar $O'$ is denoted as $\theta_p$. Since $\overrightarrow{AA'} = -\overrightarrow{A'A}$, we have an identity from the above geometries:

$$\gamma' + \theta_p - \pi = \gamma - \pi/2 + \theta_i. \tag{S1}$$

Considering the maximum length of the rod (without intersecting any pillar circumferences) as $l_{p,\max}$, we can represent the vector $\overrightarrow{AA'}$ by both $(l_{p,\max}, \gamma - \pi/2 + \theta_i)$ in polar coordinates (with respect to $A$) and $\overrightarrow{OA'} - \overrightarrow{OA}$ in Cartesian coordinates, followed by the identities:

$$l_{p,\max}\cos\big(\gamma - \pi/2 + \theta_i\big) = R\left(\frac{a}{R} + \cos\gamma' - \cos\gamma\right), \tag{S2}$$

$$l_{p,\max}\sin\big(\gamma - \pi/2 + \theta_i\big) = R\big(\sin\gamma' - \sin\gamma\big). \tag{S3}$$

Eliminating $l_{p,\max}$ from the above two equations gives

$$\tan(\gamma + \theta_i) = -\left[\frac{a}{R} + \sin\big(\theta_p - \gamma - \theta_i\big) - \cos\gamma\right] / \left[\cos\big(\theta_p - \gamma - \theta_i\big) - \sin\gamma\right] \tag{S4}$$

Letting $x \equiv \sin(\gamma') = \cos\big(\theta_p - \gamma - \theta_i\big)$ and $b \equiv \cos\gamma - \frac{a}{R} + \tan(\gamma+\theta_i)\sin\gamma$, we rewrite the above equation as a quadratic equation for $x$:

$$\big[b - \tan(\gamma + \theta_i)x\big]^2 = 1 - x^2. \tag{S5}$$

Solving this quadratic equation gives

$$x\left(\gamma, \theta_i, \frac{R}{a}\right) = \frac{b\tan(\gamma+\theta_i) \pm \sqrt{b^2\tan^2(\gamma+\theta_i) - (b^2-1)\left[1 + \tan^2(\gamma+\theta_i)\right]}}{1 + \tan^2(\gamma+\theta_i)}. \tag{S6}$$

Consequently, the cell orientation with respect to the neighboring pillar becomes

$$\theta_p = \cos^{-1} x\left(\gamma, \theta_i, \frac{R}{a}\right) + \gamma + \theta_i \tag{S7}$$

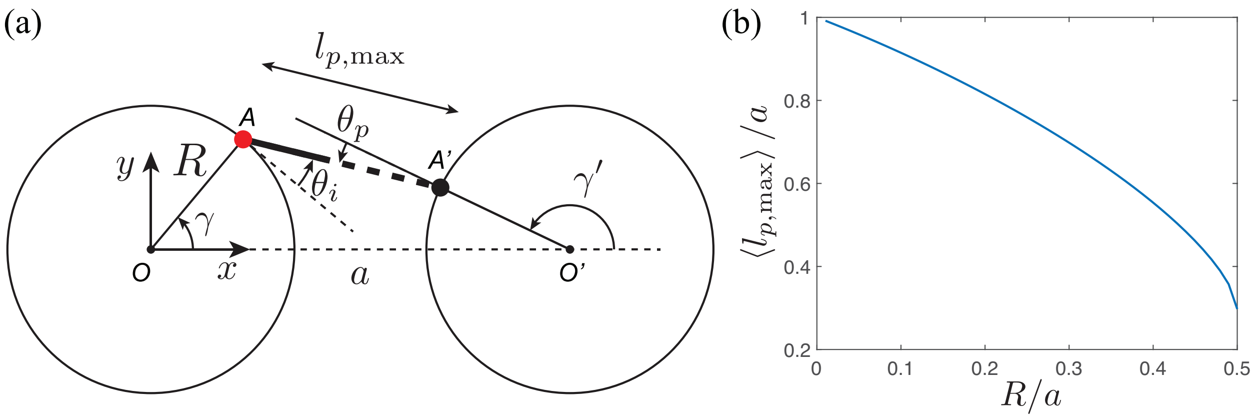


Figure S1: Geometric constraints in a pillar lattice. (a) Here, the distance between adjacent pillars is given by the lateral size of a square lattice $a = \left|\overrightarrow{OO'}\right|$. A bacterium is simplified as an infinitely thin rod up to a maximum $\left|\overrightarrow{AA'}\right|$ that circulates around a pillar at the origin $O$ along the counter-clockwise direction. The cell orientation deviates from the surface tangential by an incident angle $\theta_i$. An adjacent pillar (centered at $O'$) enhances or interrupts the circulation of the microorganisms by providing a force along its surface normal ($\overrightarrow{O'A'}$) and hence a torque. A clockwise or counter-clockwise torque is demarcated by the sign of the angle $\theta_p$, the orientation of the cell relative to the $O'$ pillar. (b) The computed mean maximum length $\langle l_{p,\max}\rangle$ (normalized by the lattice size $a$) is shown as a function of the lattice geometry, characterized by a dimensionless pillar radius $R/a$.

and the maximum length

$$l_{p,\max} = R\frac{\sin\gamma - x\left(\gamma, \theta_i, R/a\right)}{\cos\left(\gamma + \theta_i\right)} \tag{S8}$$

One of these two roots (Eq. S6) is associated with the intersection between $\overrightarrow{AA'}$ and the far side of the pillar, which can be ruled out easily by keeping the shorter $l_{p,\max}$.

Given that the incident angle is small, i.e., $\theta_i = 0$, we compute the mean of the above maximum length $l_{p,\max}$ over the angle $\gamma$ as

$$\langle l_{p,\max}\rangle = \frac{a}{\gamma_{\max} - \gamma_{\min}} \int_{\gamma_{\min}}^{\gamma_{\max}} \left(\frac{R}{a}\right) \frac{\sin\gamma - x\left(\gamma, 0, R/a\right)}{\cos\gamma} \mathrm{d}\gamma, \tag{S9}$$

where $\gamma_{\min}$ and $\gamma_{\max}$ are the lower and upper bounds for real integrand within one quadrant, which are evaluated numerically in MatLab. The dependency of $\langle l_{p,\max}\rangle$ on lattice geometries ($R/a$) are shown in Fig. S1b. Example values for selected geometries, especially those of the interest in this study, are enumerated in Supplementary Table S1.

Table S1: Mean maximum pusher sizes $\langle l_{p,\max}\rangle$ computed for different lattice geometries $R/a$.

| $R/a$ | $\langle l_{p,\max}\rangle /a$ |
|---|---|
| 0.100 | 0.915 |
| 0.333 | 0.654 |
| 0.375 | 0.595 |
| 0.417 | 0.525 |
| 0.500 | 0.297 |

## Agent-based kinematics

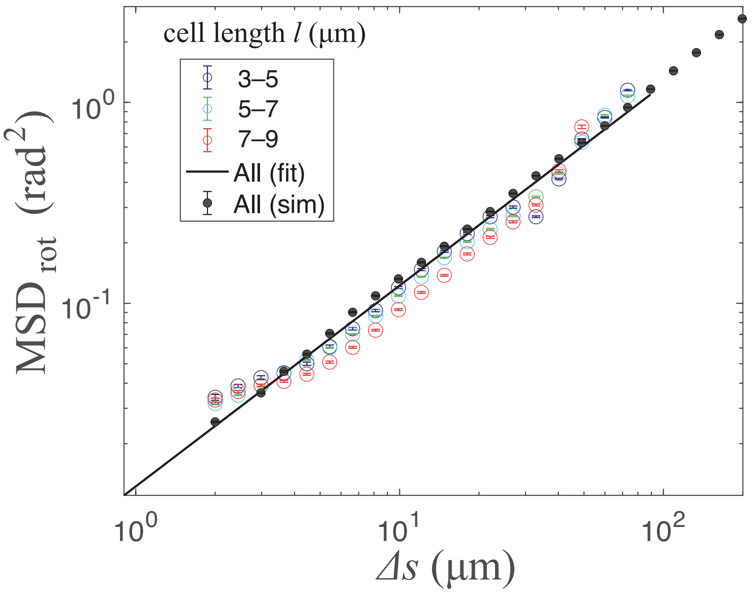


Figure S2: The rotational diffusion of free-swimming bacteria. The angular mean-squared displacement ($\mathrm{MSD}_{\mathrm{rot}}$) of the swimming directions of *E. coli* is shown against the elapsed path length $\Delta s$ for different cell body lengths (open circles). A rotational diffusion coefficient ($D_{\mathrm{rot}} = \frac{1}{2}\mathrm{MSD}_{\mathrm{rot}}/\Delta s$) is obtained by a proportional fit (solid line) of $\mathrm{MSD}(\Delta s)$ for all cell body lengths, yielding a random-walk step in cell orientation to be used in the agent-based simulation. The simulated trajectory of free-swimming cells with the above extracted random-walk step reproduces the same rotational diffusivity (dots).

To apply these geometry-based pillar effects to cell kinematics, we neglect the slight dependency of the locations of the attractive and repulsive zones on the circulation directions (Fig. 3) and focus on a deterministic residency within each attractive zone and a probabilistic residency within each repulsive zone. In the repulsive case, we assume that the cell can either reside on the pillar surface throughout the entire repulsive zone or leave immediately upon entering that zone, determined by comparing a numerically generated random number (uniformly distributed between 0 and 1) with the given escaping probability $P_{\mathrm{esc}}$. Once the cell escapes, we prescribe its swimming direction along the tangential direction of its previously orbited pillar. A white noise of small amplitude is applied to swimming directions afterwards to account for a rotational diffusion in the free-swimming direction of the non-tumbling mutant, which is extracted from the experimental trajectories (Fig. S2).

To characterize such rotational diffusivities in experiments, we computed the angular mean-squared displacement ($\mathrm{MSD}_{\mathrm{rot}} = \langle(\theta - \langle\theta\rangle)^2\rangle$) from the swimming directions $\theta$, and showed it as a function of the elapsed path length $\Delta s$. Results for different cell lengths are similar (Fig. S2). A proportional fit of the data for all cell sizes gives a rotational diffusion coefficient $D_{\mathrm{rot}} = \mathrm{MSD}_{\mathrm{rot}}/(2\Delta s) \approx 0.0061\mathrm{rad}^2/\mu\mathrm{m}$. Given the typical step size in path lengths used in our simulations $\mathrm{d}s = 0.02 \times a$ (or $\mathrm{d}s = 0.8$ $\mu$m for lattice size $a = 40$ $\mu$m), we have a random-walk step in the white noise as $\mathrm{d}\theta = \pm\sqrt{D_{\mathrm{rot}}\mathrm{d}s/2} \approx \pm 0.05$ rad. Not surprisingly, applying this white noise to the simulation of free-swimming bacteria (without pillars) restores the same rotational diffusivities (Fig. S2).

We prescribe the attractive zones ($\theta_p > 0$ or without nearest-pillar constraints) from the calculation in the previous section. For simplicity, we consider $\theta_i = 0$ and use the averaged attractive zones from both the clockwise and the counter-clockwise cases. These averaged attractive zones are thus centered at $\gamma = 0$, $\pi/2$, $\pi$, and $3\pi/2$ with respect to the center of the orbited pillar. Each agent starts at a randomly generated position and moves at a constant speed. Within the vicinity of the pillar surface (determined by the criterion that the distance to pillar center $O$ is shorter than the $O$ pillar radius), the agent either keeps staying on the

pillar surface through circulation or leaves the surface along the tangential direction. Such binary activities are determined by whether the agent is within the repulsive ($\theta_p < 0$) or the attractive (otherwise) zones: the agent leaves the pillar with a probability $P_{\text{esc}}$ within the repulsive zone or moves along the circumference of the pillar until it reaches the next repulsive zone.

The MatLab code that simulates such a process is shared through GitHub: `https://github.com/liubiofluids/geometricpillar`.

## Stochastic escaping model

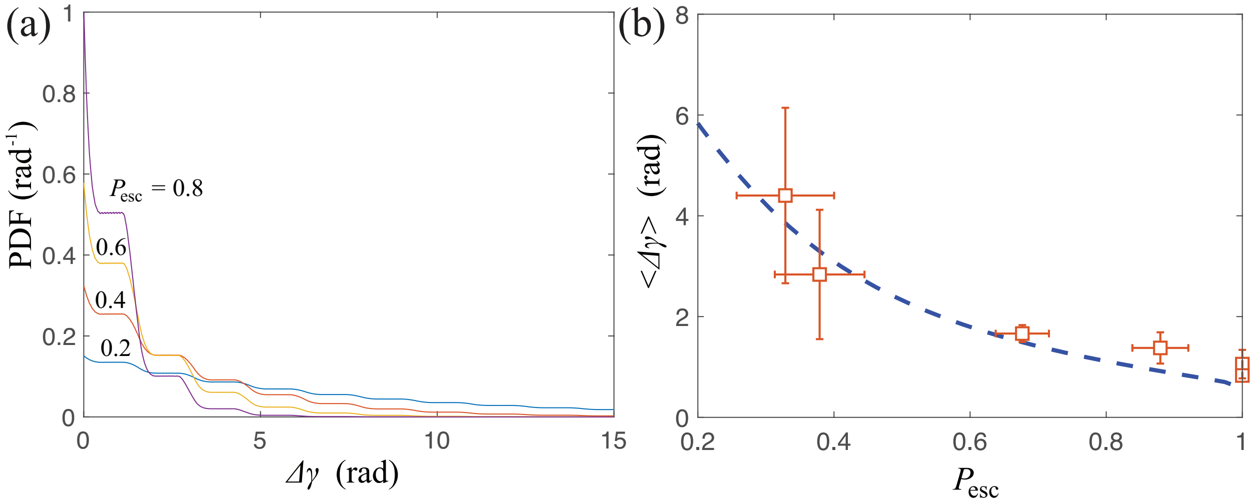


Figure S3: Stochastic escaping of bacteria from pillar surfaces. (a) Probability density functions of residency arc angles $\Delta\gamma$ for various escaping probabilities within the repulsive zones $P_r = P_{\text{esc}}$, as predicted by a stochastic process (Eq. S15). Here, the escaping probability within the attractive zones is prescribed to be $P_a = 0$ and the distribution curves are averaged for $\gamma_i \in [0, \pi/2)$. (b) The resulting mean residency arc angles $\langle\Delta\gamma\rangle$ are shown as a function of $P_{\text{esc}}$ (dashed line). The experimental data (squares, with all error bars indicating standard errors) are shown for comparison.

We consider a random process with the bacterium leaving its previously orbited pillar only within any repulsive zones at a uniform probability $P_{\text{esc}}$. The probability of finding a residency arc angle $\Delta\gamma$ can thus be represented by a Bernoulli process [3] as

$$p(\Delta\gamma) = (1 - P_{\text{esc}})^{n_r} P_{\text{esc}}, \tag{S10}$$

where $n_r$ is the number of repulsive zones that the bacterium passes without exiting its circulation, i.e.,

$$n_r = \begin{cases} \left[ \left| |\gamma_f - \gamma_i| - \Delta\gamma_0 \right| / (\pi/2) \right], & \text{if } \gamma_i \in \text{any repulsive zones} \\ [|\gamma_f - \gamma_i|/(\pi/2)], & \text{if otherwise.} \end{cases} \tag{S11}$$

Here, $\gamma_i$ and $\gamma_f$ are respectively the initial and final angular position of a circulation, $\Delta\gamma_0$ is the size of an attractive zone (Fig. 3), and the symbol $[\cdot]$ corresponds to the integer part of a number. It is worth noting that the model so far ignores the detailed position where a bacterium enters ($\gamma_i$) or leaves ($\gamma_f$) the pillar surfaces and the potential finite escaping probability within the attractive zones. Given the binary escaping probabilities within attractive and repulsive zones ($P_a$ and $P_r$ respectively), we show in the following that the above result can be further generalized to a more realistic escaping model. For simplification in the derivation, we represent the probability that a bacterium moves along the pillar surface for a small angular

displacement $\delta\gamma$ by $p_{a,r} = e^{-\nu_{a,r}\delta\gamma}$, with index $a$ or $r$ denoting the type of zones (attractive or repulsive, respectively). Matching the probability that a bacterium escapes within a single attractive $P_a$ or repulsive zone $P_r$, we have

$$P_{a,r} = \sum_{j=1}^{N_{a,r}} e^{-j\nu_{a,r}\delta\gamma} \left(1 - e^{-\nu_{a,r}\delta\gamma}\right), \tag{S12}$$

where $N_{a,r}$ is the number of discretized angle elements $\delta\gamma$ within an attractive ($N_a$) or a repulsive ($N_r$) zone. We thus have in the continuum limit

$$P_{a,r} \xrightarrow{\delta\gamma\to 0} 1 - e^{-\nu_{a,r}\Delta\gamma_{a,r}}, \tag{S13}$$

or

$$\nu_{a,r} = -\ln(1 - P_{a,r})/\Delta\gamma_{a,r}, \tag{S14}$$

where $\Delta\gamma_{a,r}$ is the size of a single attractive or repulsive zone, i.e., $\Delta\gamma_a = \Delta\gamma_0$ and $\Delta\gamma_a = \pi/2 - \Delta\gamma_0$. The probability density function $p(\Delta\gamma)$ of a bacterium to circulate about the pillar for an arbitrary $\Delta\gamma$ is given by

$$p(\Delta\gamma)\mathrm{d}\Delta\gamma = (1 - P_a)^{n_a}(1 - P_r)^{n_r}\nu_{a,r}\mathrm{d}\Delta\gamma, \tag{S15}$$

where $n_{a,r}$ are multiples (as real numbers) of attractive or repulsive zones covered in the circulation, and the index ($a$ or $r$) of $\nu$ is determined by the type of zones where the bacterium escapes. This probability distribution thus depends not only on the residency arc angle $\Delta\gamma$ but also on the detailed location of $\gamma_i$ and $\gamma_f$ within the attractive and repulsive zones. Not surprisingly, for isotropic escaping ($P_a = P_r$ and $\nu_a = \nu_r$), our result becomes $p(\Delta\gamma) = \nu_r e^{-\nu_r\Delta\gamma}$, recovering a classic Poisson process.

Examples of such distribution functions (averaged for all possible $\gamma_i$) are computed and shown in Fig. S3(a). We also computed the corresponding mean residency arc angles $\langle\Delta\gamma\rangle$, which show a decent agreement with the experimental observations (Fig. S3(b)).

## Supporting data for the geometric effects due to pillar lattices

The size-dependent distributions of bacteria near pillar surfaces (shown in Fig. 2b and 2c) can be further illustrated by averaging the concentrations $\rho$ along angular directions $\gamma$ and showing the corresponding radial distributions $\langle\rho\rangle_\gamma$. These radial distributions normalized by a uniform density $\rho_0$ are shown in Fig. S4(a). Again, the concentration of the shorter cells ($l < 5$ $\mu$m) near the pillar surfaces (denoted by the shaded area) are much higher than that of the longer cells ($l > 7$ $\mu$m), consistent with the geometry-induced escaping for longer cells. In addition to the heterogeneity along the radial direction, the distribution of bacteria near a pillar is anisotropic. Figure S4(b) shows such a fluctuated cell concentration along a pillar's annulus. The peaks of the fluctuation coincide with location of the attractive zones as predicted by the above geometric model, consistent with the neighboring-pillar effects.

A volume exclusion due to the finite cell body size can potentially cause a size-dependent distribution of bacteria near pillar surfaces similar to what we observed experimentally (Fig. 2b and 2c). If that is the case, the front of cell body will be closer to the pillar center than its center. As shown in Fig. S5, both the center and the front of the cell body show a similar radial distribution within one unit cell, which rules out the potential contribution of volume exclusion to the size-dependent effect that we observed.

To validate the geometric effects due to neighboring pillars, we examined the residency of *E. coli* on pillar surfaces in an extreme array geometry with its lattice size $a = 70$ $\mu$m while retaining the same pillar radii ($R = 15$ $\mu$m). The gap between any adjacent pillars becomes $d = a - 2R = 40$ $\mu$m, much longer than the longest cell observed in this study. Here, we focus on the residency angles $\Delta\gamma$. Compared to the short gap

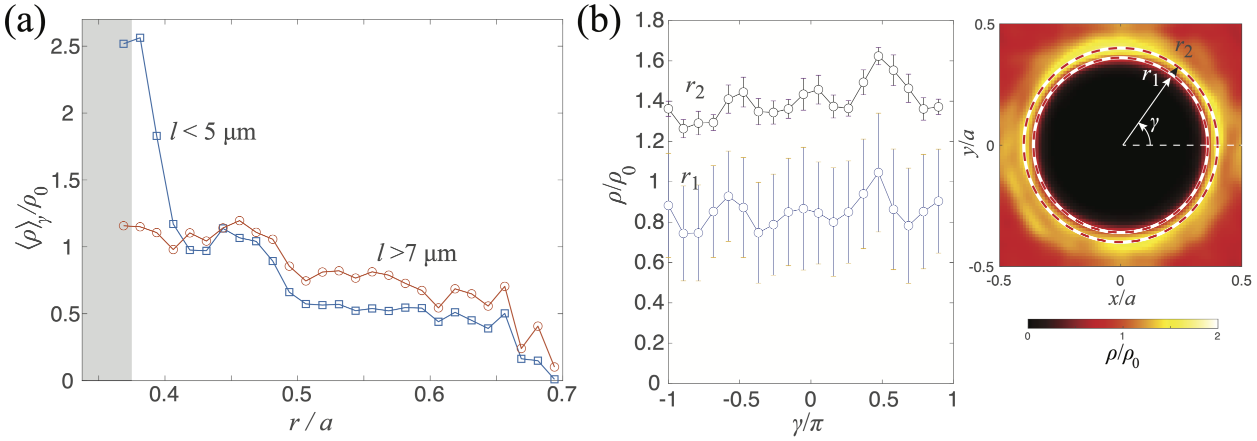


Figure S4: Heterogeneous cell concentrations near pillar surfaces. (a) The averaged radial distribution of *E. coli* (Fig. 2b and 2c) shows a higher concentration adjacent to pillar surfaces for shorter cells. The shaded area corresponds to the pillar region (with its radius $R = 0.375a$). (b) Distribution $\rho$ is shown as function of the angular position $\gamma$ about a pillar at different radii ($r_1$ and $r_2$) for the same pillar geometry ($R = 0.375a$). The inset shows the locations of these radii in the corresponding 2D distribution of *E. coli* (with their cell body lengths 2 $\mu$m $< l <$ 7 $\mu$m). All distributions here are normalized by their values in the uniform case, $\rho_0$.

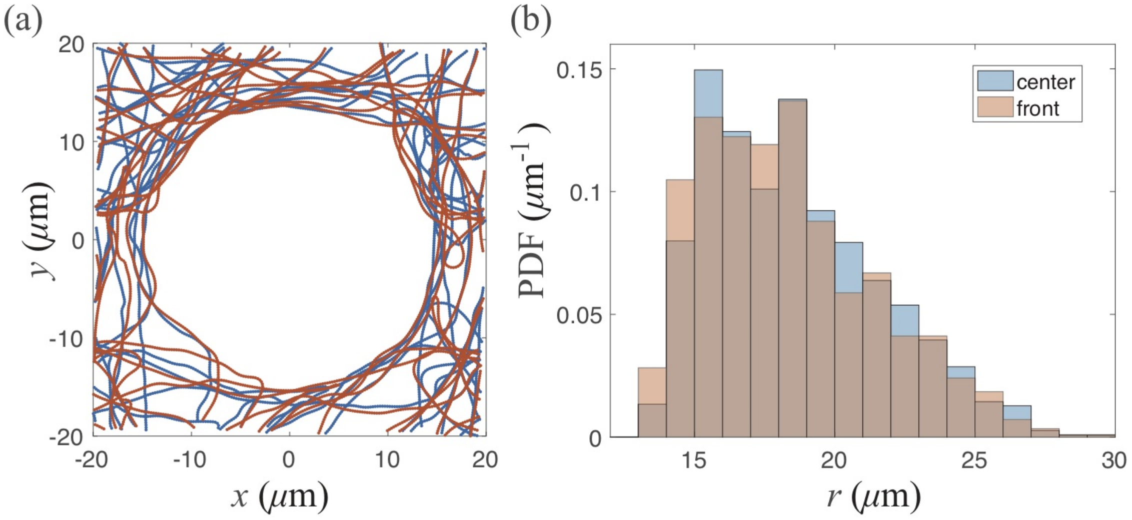


Figure S5: Potential volume exclusion effect (due to finite cell lengths) in the bacterial distribution near the pillar surface. (a) Two example trajectories of the same *E. coli* cell are obtained by tracking the center of the cell body (blue) and its front (red). Both trajectories are mapped into one unit cell of the pillar lattice ($a = 40$ $\mu$m, $R = 15$ $\mu$m). (b) The probability distribution functions (PDF) from these trajectories are shown as a function of the distance to the pillar center ($r$). Here the length of the cell body is $5.8 \pm 0.2$ $\mu$m.

($d = 10$ $\mu$m) case, the size-dependency in bacterial residency on pillar surfaces vanishes within the range of cell body lengths in this study (Fig. S6). The relatively longer cells ($l > 7$ $\mu$m) that are previously unable to circulate around any pillars ($\Delta\gamma \lesssim \pi$ at $d = 10$ $\mu$m) can now circulate over multiple turns with this increased gap size ($d = 40$ $\mu$m). However, the variation in residency (due to this new gap size) is insignificant for relatively shorter cells ($l < 4$ $\mu$m). These results thus suggest a constraint of neighboring pillars on bacteria circulation that is sensitive to the relative size of bacteria (including cell bodies and flagella) compared to pillar gaps and thus further validate our geometric model.

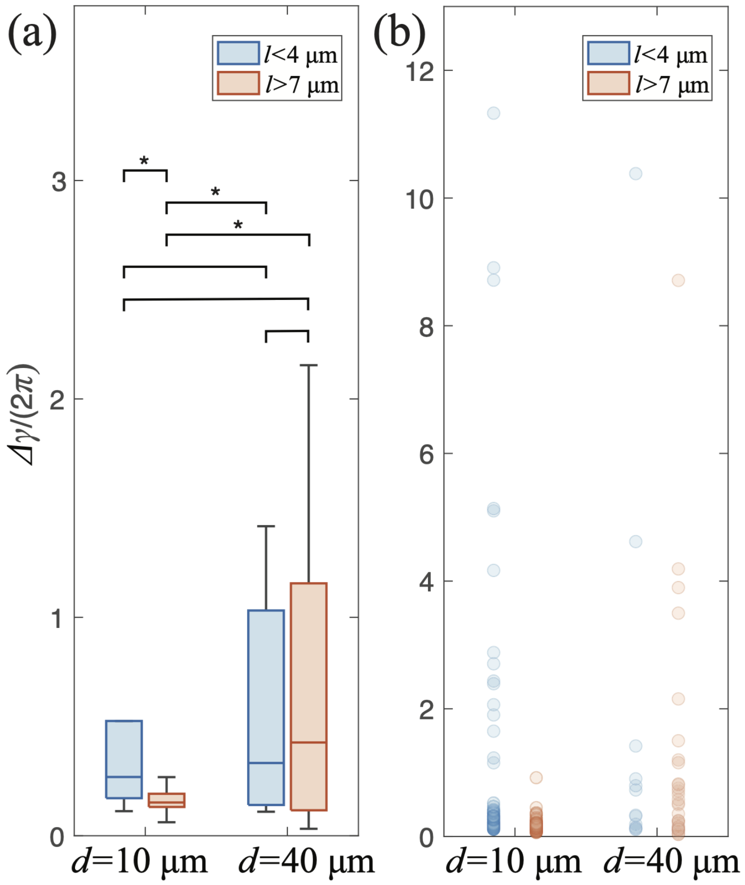


Figure S6: Validating the neighboring-pillar effects on size-dependent bacterial trapping. (a) The box plots of the residency angles $\Delta\gamma$ of *E. coli* (normalized by a full turn $2\pi$) are shown for both short ($l < 4$ $\mu$m) and long cells ($l > 7$ $\mu$m) under two sets of pillar geometries (with gaps between adjacent pillars $d = 10$ and 40 $\mu$m). With this increased gap, the resident angles for long cells are significantly higher while the difference for short cells is insignificant. An asterisk ('*') above the link between two data sets indicates a significant difference (here, with its $p$-value $< 10^{-3}$) from a two-sample t-test (with a Kolmogorov–Smirnov test showing the same result). (b) The corresponding residency angles for the box plots shown in (a) also illustrates a suppressed trapping for long cells ($l > 7$ $\mu$m) when subjected to small pillar gaps ($d = 10$ $\mu$m). The sample size of each column of data (from left to right) is 66, 85, 13, and 34, respectively.

The circulation of bacteria that we observed here is also distinguishable from those circular motions of bacteria subjected to a nearby solid surface [4]. In those surface-induced circulations, the direction of circulation is pertinent to the flagellar chirality and is thus unidirectional. For instance, the circulation of *E. coli* near a bottom coverslip is always in the clockwise direction (viewed from the top) due to left-handed flagella. However, in a micropillar array, a bacterium can circulate around a pillar in either direction, depending on its initial orientation when approaching the pillar surface. Figure S7 shows such a bidirectional circulation of bacteria around micro-pillars. In addition to the bistability, the dominating curvatures in a pillar-induced circulation also match the pillar radii, which is distinct from the circulation next to a nearby surface.

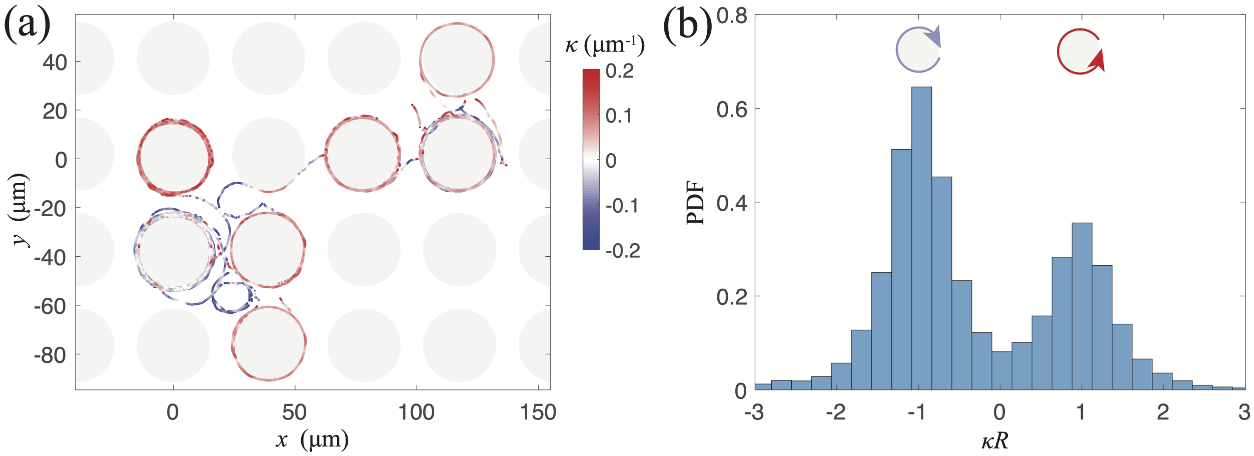


Figure S7: Bi-directional circulation of bacteria around pillar surfaces. (a) As shown by the local curvature $\kappa$ of the trajectory, the same bacterium can circulate a micropillar in both clockwise (blue) and counter-clockwise directions (red), as viewed from the top. (b) The probability density function of the normalized curvature $\kappa R$ (sampled every 0.2 $\mu$m along the path) shows such a bistability in circulation directions. The slight asymmetry in the distribution is potentially subjected to a nearby bottom surface, which leads more stable clockwise circulations.

## Bacterial culturing and sample visualization

The *E. coli* strain (HCB437) was grown on a plate (4% tryptic soy agar) at 30°C after inoculation. One motile colony from the plate was transferred to a flask with 10 mL tryptic soy broth (4% tryptic soy broth), incubated on an orbital shaker (running at 200 RPM) for 16 hr at 30°C. The sample was then diluted 500 times with tryptic soy broth and incubated for another 3.5 hr at 30°C in the shaker incubator (at 200 RPM). After incubation, the sample was diluted 50 times, followed by a washing process: the sample was centrifuged (at 2000 RPM for 4 min) and re-suspended in a motility buffer (0.064 M $K_2HPO_4$, 0.035 M $KH_2PO_4$, 0.078 mM EDTA, 0.067 M NaCl, pH =7) for 3 times before being prepared as a specimen.

The micropillar arrays were fabricated through a standard soft photolithography approach [5]. The pillar lattices were generated by a computer-aided design (CAD) software and imprinted on a soda-lime glass mask (Photronics) for UV photolithography. A negative photoresist (SU-8 2015, Kayaku Advanced Materials Inc.) was applied to create a master (of 30 $\mu$m thick) for molding the polydimethylsiloxane (PDMS) pillars (of 30 $\mu$m in heights).

Individual cells were visualized under an inverted microscope (Nikon Eclipse Ti) at a 60× magnification, recorded at 208 fps by a video camera (Allied Vision Pike F-032B). Our self-programmed software played back the high-speed video in real time and controlled the 3-axis microscope stages (Physik Instrumente PINano Piezo XYZ Stage $70 \times 70 \times 50$ $\mu$m and Prior Scientific XY Stage $100 \times 75$ mm) through a USB DAQ (National Instruments USB-6211) and two stepper motor controllers (Phidgets PhidgetStepper Bipolar HC) at 100 Hz for real-time tracking. In the presence of a nearby pillar surface, a manual control of the microscope stages using keyboards was applied to assist the computer-automated tracking for better tracking results. To reconstruct the full trajectories, the images of bacteria were stitched together based on the positions of all pillars in the background. Individual bacteria were tracked up to 23 minutes with the average duration of (∼100) individual trajectories $1.6 \pm 3.0$ min (mean ± S.D.) for the typical pillar lattice ($a = 10$ $\mu$m and $R = 15$ $\mu$m). The corresponding size and speed of cells in this study are shown in Fig. S8.

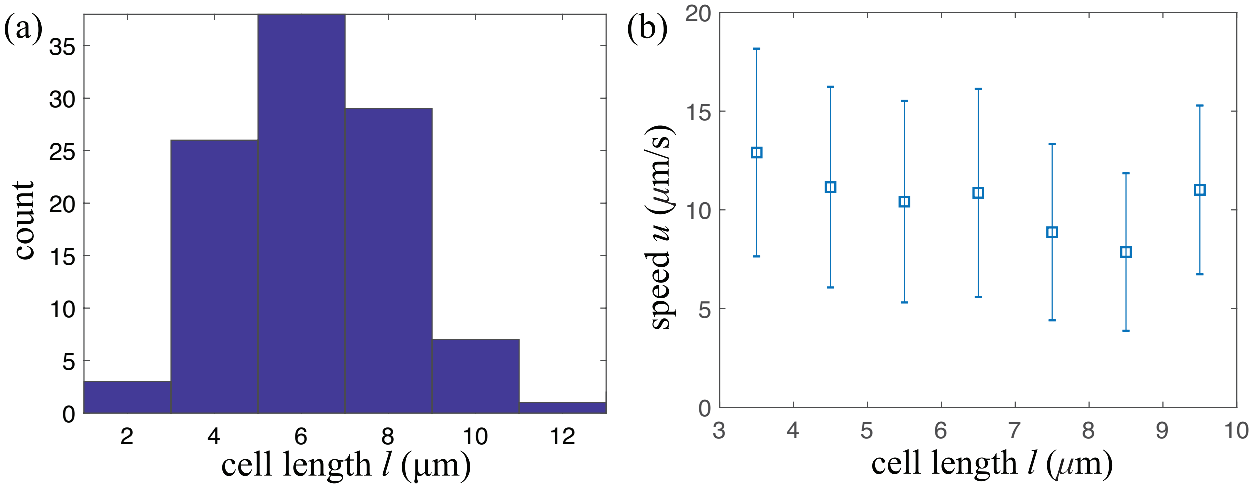


Figure S8: Size and speed variations among individual cells. (a) The histogram of cell body lengths of bacteria observed in the study of a typical pillar lattice ($R = 30$ $\mu$m and $a = 40$ $\mu$m). (b) Swimming speed of *E. coli* in pillar arrays show no significant cell length ($l$) dependencies. Error bars correspond to standard deviations.


[1] Spagnolie, S. E., Moreno-Flores, G. R., Bartolo, D. & Lauga, E. Geometric capture and escape of a microswimmer colliding with an obstacle. *Soft Matter* **11**, 3396–3411 (2015).

[2] Sipos, O., Nagy, K., Di Leonardo, R. & Galajda, P. Hydrodynamic trapping of swimming bacteria by convex walls. *Physical Review Letters* **114**, 258104 (2015).

[3] Feller, W. *An introduction to probability theory and its applications, Vol 1.* Wiley series in probability and mathematical statistics (Jon Wiley & Sons, New York, 1968), third ed. rev edn.

[4] Lauga, E., DiLuzio, W. R., Whitesides, G. M. & Stone, H. A. Swimming in circles: Motion of bacteria near solid boundaries. *Biophysical Journal* **90**, 400–412 (2006).

[5] McDonald, J. C. *et al.* Fabrication of microfluidic systems in poly(dimethylsiloxane). *Electrophoresis* **21**, 27–40 (2000).

# Description of Supplementary Videos

Movie S1. Trapping of a relatively shorter bacterium *Escherichia coli* to pillar surfaces in a square lattice (magnified at 60×). Here, the length of the cell body is $l = 4.9 \pm 0.2$ $\mu$m. The radii of pillars are $R = 15$ $\mu$m and the lateral size of the pillar lattice is $a = 40$ $\mu$m.

Movie S2. Escaping of a relatively longer bacterium *E. coli* from pillar surfaces (magnified at 60×). Here, the length of the cell body is $l = 7.5 \pm 0.1$ $\mu$m. The radii of pillars are $R = 15$ $\mu$m and the lateral size of the pillar lattice is $a = 40$ $\mu$m. The microscopic images were captured at a 60× magnification.
